# Supplementary material for: UNetFormer: A Unified Vision Transformer Model and Pre-Training Framework for 3D Medical Image Segmentation
Source: arXiv:2204.00631 source file (2022-04-05)
Supplement: Supplementary file 1 [file samplepaper.tex]

% This is samplepaper.tex, a sample chapter demonstrating the
% LLNCS macro package for Springer Computer Science proceedings;
% Version 2.21 of 2022/01/12
%
\documentclass[runningheads]{llncs}
\usepackage[T1]{fontenc}
% T1 fonts will be used to generate the final print and online PDFs,
% so please use T1 fonts in your manuscript whenever possible.
% Other font encondings may result in incorrect characters.
%
\usepackage{graphicx}
% Used for displaying a sample figure. If possible, figure files should
% be included in EPS format.
%
% If you use the hyperref package, please uncomment the following two lines
% to display URLs in blue roman font according to Springer's eBook style:
%\usepackage{color}
%\renewcommand\UrlFont{\color{blue}\rmfamily}
%
\begin{document}
\title{Contribution Title\thanks{Supported by organization x.}}
%
%\titlerunning{Abbreviated paper title}
% If the paper title is too long for the running head, you can set
% an abbreviated paper title here
%
\author{First Author\inst{1}\orcidID{0000-1111-2222-3333} \and
Second Author\inst{2,3}\orcidID{1111-2222-3333-4444} \and
Third Author\inst{3}\orcidID{2222--3333-4444-5555}}
\authorrunning{F. Author et al.}
% First names are abbreviated in the running head.
% If there are more than two authors, 'et al.' is used.
%
\institute{Princeton University, Princeton NJ 08544, USA \and
Springer Heidelberg, Tiergartenstr. 17, 69121 Heidelberg, Germany
\email{lncs@springer.com}\\
\url{http://www.springer.com/gp/computer-science/lncs} \and
ABC Institute, Rupert-Karls-University Heidelberg, Heidelberg, Germany\\
\email{\{abc,lncs\}@uni-heidelberg.de}}
\maketitle              % typeset the header of the contribution
\begin{abstract}
The abstract should briefly summarize the contents of the paper in
150--250 words.

\keywords{First keyword  \and Second keyword \and Another keyword.}
\end{abstract}
\section{First Section}
\subsection{A Subsection Sample}
Please note that the first paragraph of a section or subsection is
not indented. The first paragraph that follows a table, figure,
equation etc. does not need an indent, either.

Subsequent paragraphs, however, are indented.

\subsubsection{Sample Heading (Third Level)} Only two levels of
headings should be numbered. Lower level headings remain unnumbered;
they are formatted as run-in headings.

\paragraph{Sample Heading (Fourth Level)}
The contribution should contain no more than four levels of
headings. Table~\ref{tab1} gives a summary of all heading levels.

\begin{table}
\caption{Table captions should be placed above the
tables.}\label{tab1}
\begin{tabular}{|l|l|l|}
\hline
Heading level &  Example & Font size and style\\
\hline
Title (centered) &  {\Large\bfseries Lecture Notes} & 14 point, bold\\
1st-level heading &  {\large\bfseries 1 Introduction} & 12 point, bold\\
2nd-level heading & {\bfseries 2.1 Printing Area} & 10 point, bold\\
3rd-level heading & {\bfseries Run-in Heading in Bold.} Text follows & 10 point, bold\\
4th-level heading & {\itshape Lowest Level Heading.} Text follows & 10 point, italic\\
\hline
\end{tabular}
\end{table}

\noindent Displayed equations are centered and set on a separate
line.
\begin{equation}
x + y = z
\end{equation}
Please try to avoid rasterized images for line-art diagrams and
schemas. Whenever possible, use vector graphics instead (see
Fig.~\ref{fig1}).

\begin{figure}
\includegraphics[width=\textwidth]{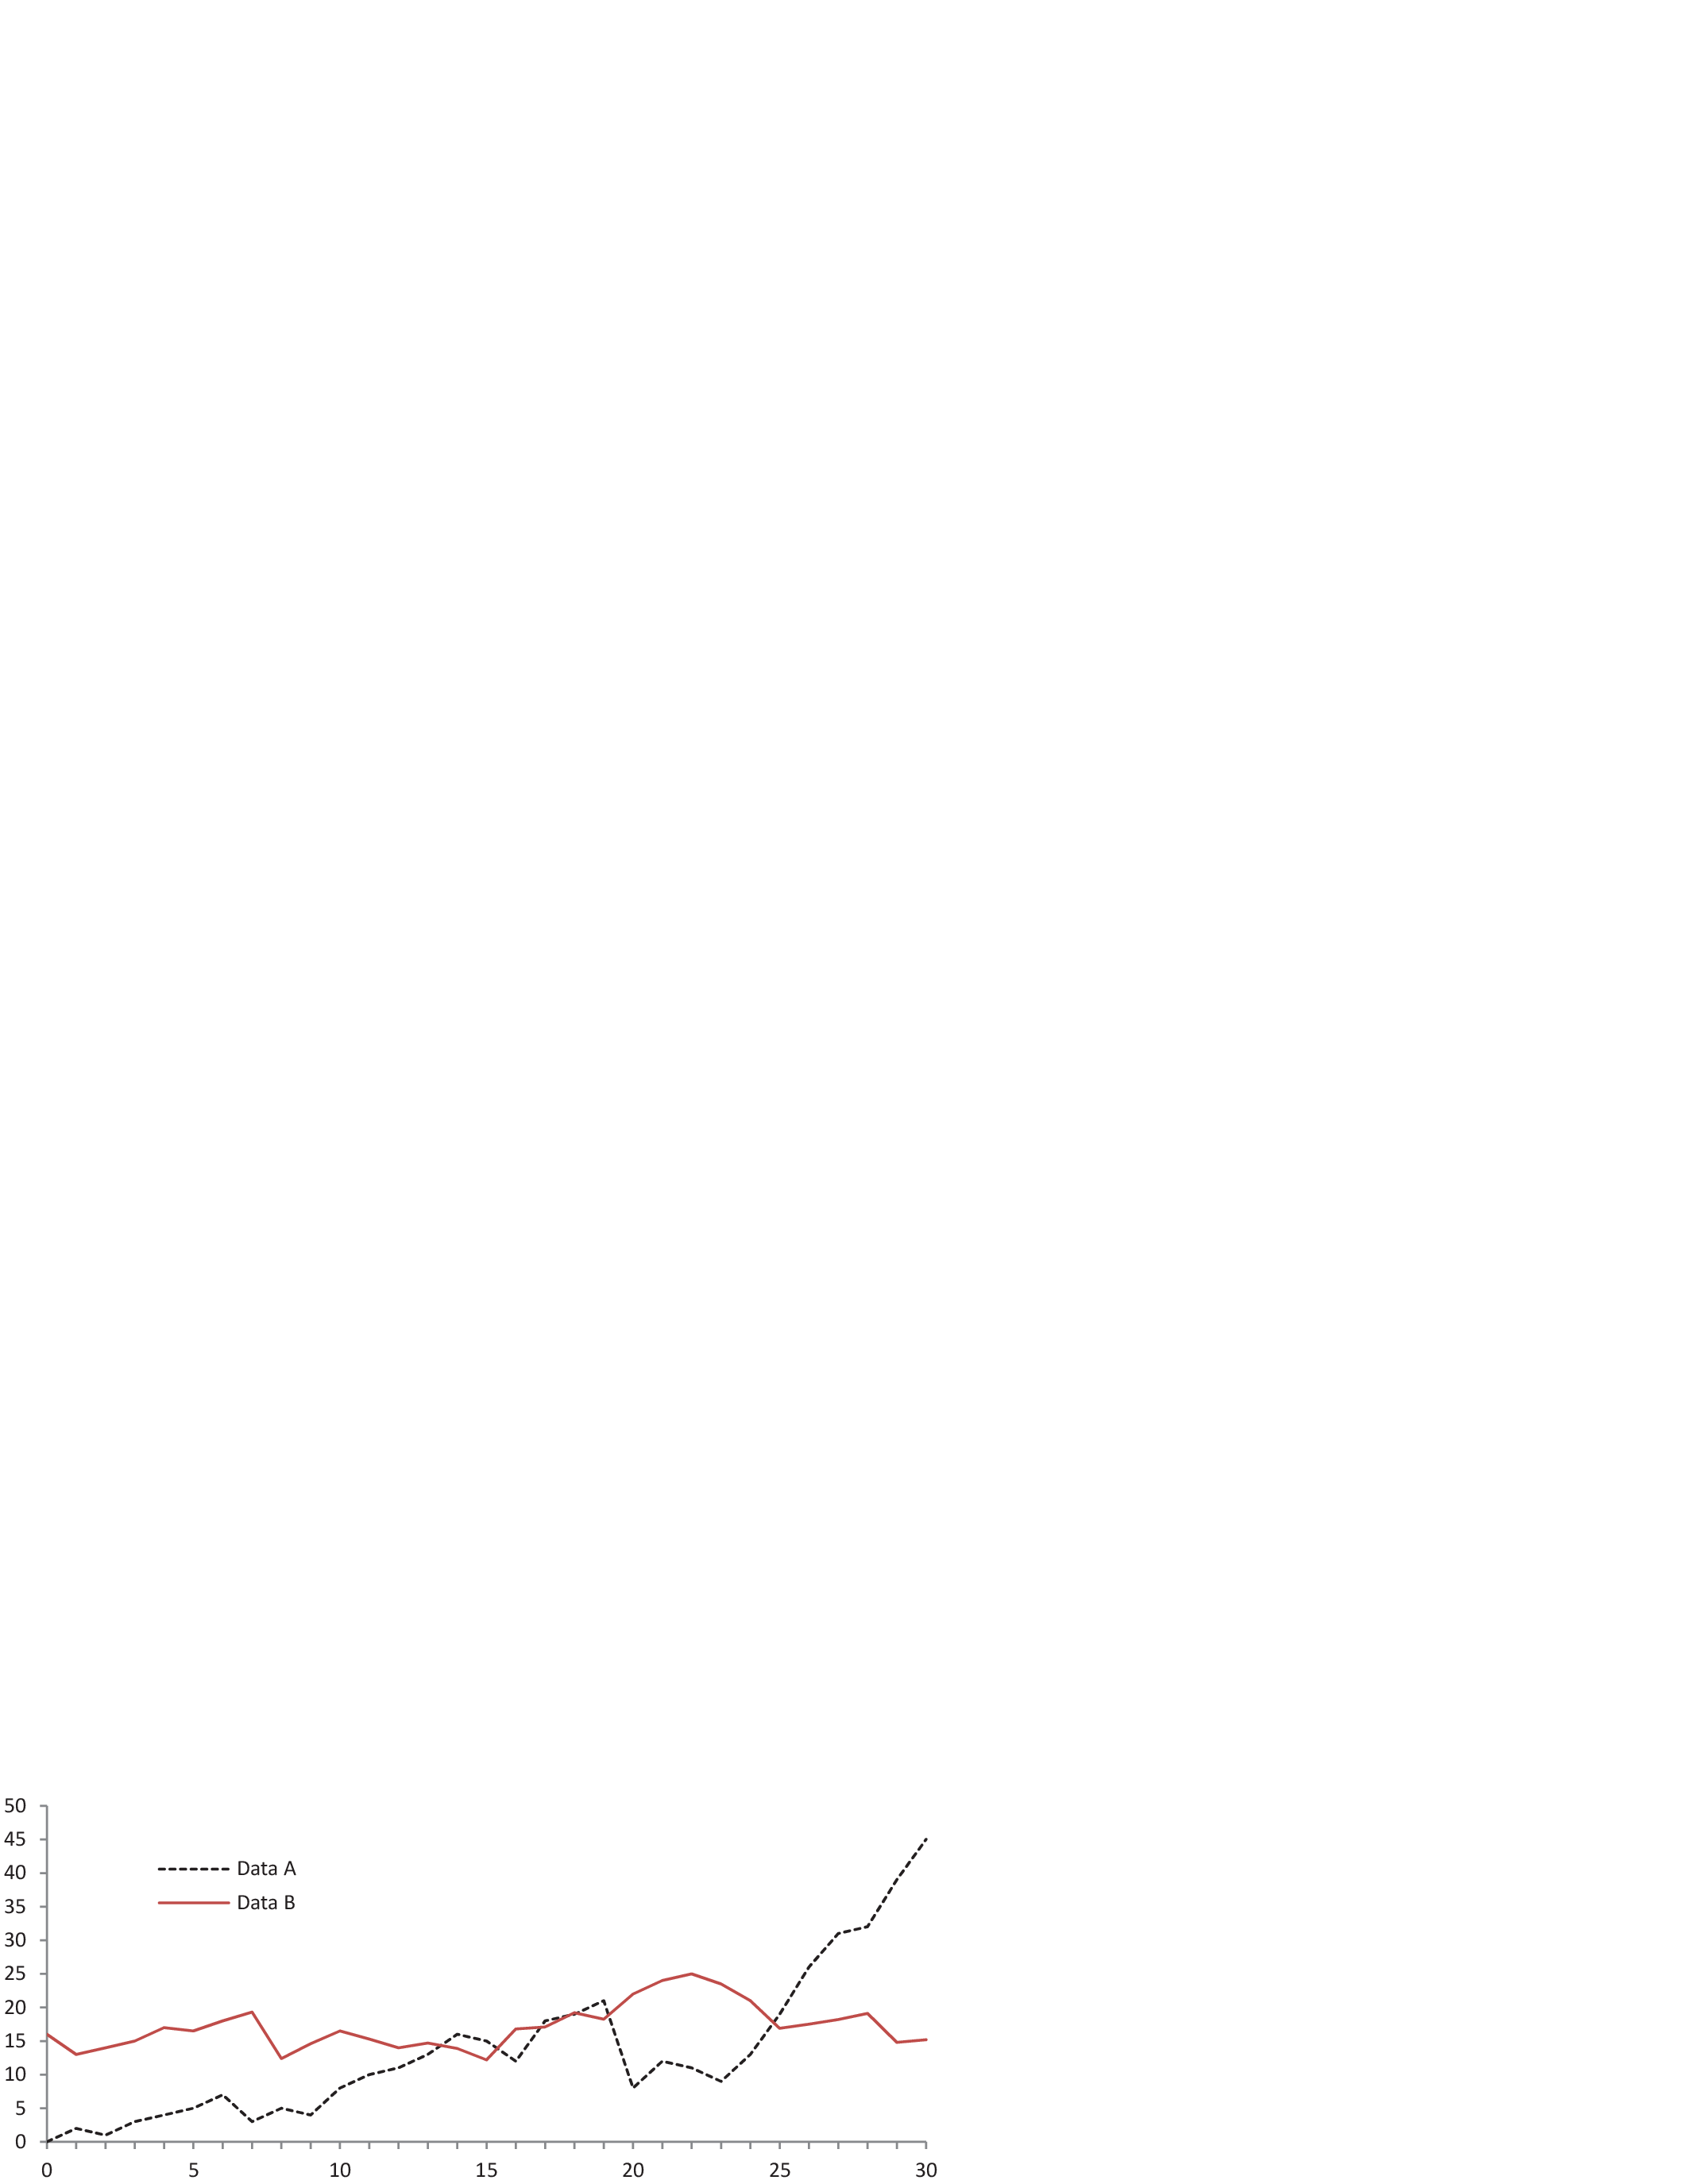}
\caption{A figure caption is always placed below the illustration.
Please note that short captions are centered, while long ones are
justified by the macro package automatically.} \label{fig1}
\end{figure}

\begin{theorem}
This is a sample theorem. The run-in heading is set in bold, while
the following text appears in italics. Definitions, lemmas,
propositions, and corollaries are styled the same way.
\end{theorem}
%
% the environments 'definition', 'lemma', 'proposition', 'corollary',
% 'remark', and 'example' are defined in the LLNCS documentclass as well.
%
\begin{proof}
Proofs, examples, and remarks have the initial word in italics,
while the following text appears in normal font.
\end{proof}
For citations of references, we prefer the use of square brackets
and consecutive numbers. Citations using labels or the author/year
convention are also acceptable. The following bibliography provides
a sample reference list with entries for journal
articles~\cite{ref_article1}, an LNCS chapter~\cite{ref_lncs1}, a
book~\cite{ref_book1}, proceedings without editors~\cite{ref_proc1},
and a homepage~\cite{ref_url1}. Multiple citations are grouped
\cite{ref_article1,ref_lncs1,ref_book1},
\cite{ref_article1,ref_book1,ref_proc1,ref_url1}.

\subsubsection{Acknowledgements} Please place your acknowledgments at
the end of the paper, preceded by an unnumbered run-in heading (i.e.
3rd-level heading).

%
% ---- Bibliography ----
%
% BibTeX users should specify bibliography style 'splncs04'.
% References will then be sorted and formatted in the correct style.
%
% \bibliographystyle{splncs04}
% \bibliography{mybibliography}
%

\end{document}
